# Supplementary material for: MCA-based Rule Mining Enables Interpretable Inference in Clinical Psychiatry
Source: arXiv:1810.11558 source file (2018-12-16)
Supplement: Supplementary file 1 [file supplementary.tex]

\section{SUPPLEMENTARY MATERIAL}

\todo{Placeholder}.
Use this space for initial submission.
For final submission this material becomes a separate document.
